# Supplementary material for: ViTCoD: Vision Transformer Acceleration via Dedicated Algorithm and Accelerator Co-Design
Source: arXiv:2210.09573 source file (2025-03-03)
Supplement: Supplementary file 1 [file 6-Appendix.tex]

\newpage
% \appendix
\begin{appendices}
\onecolumn
% \twocolumn

\section{Summarize the Major Revise}

\begin{itemize}
    \item Add roofline model to articulate the memory/bandwidth bound due to sparsity
    \begin{itemize}
        \item \textbf{Where}: Fig. \ref{fig:roofline} and Sec. \ref{sec:intro}
        \item \textbf{Who}: Reviewer-A/C-Q1; Reviewer-B-Q3; Reviewer-C-Q4; Reviewer-D-Q2/Q3; 
    \end{itemize}
    
    \item Properly position this work w.r.t. related works. Add taxonomy table to distill the field for the readers.
    \begin{itemize}
        \item \textbf{Where}: Table \ref{tab:taxonomy} and Sec. \ref{sec:related_works}
        \item \textbf{Who}: Reviewer-B-Q12; Reviewer-C-Q2;
    \end{itemize}
    
    \item Clarify experiment setups in Fig. \ref{fig:comp_alg}, \ref{fig:ae_levit}, and \ref{fig:comp_accelerator}.
    \begin{itemize}
        \item \textbf{Where}:Sec. \ref{sec:alg_exps} and Sec. \ref{sec:hardware_exps}.
        \item \textbf{Who}: Reviewer-A-Q2;
    \end{itemize}
    
    \item Clarify why ViTCoD achieves more than 2$\times$ end-to-end speedups.
    \begin{itemize}
        \item \textbf{Where}: Sec. \ref{sec:overall_comp}
        \item \textbf{Who}: Reviewer-B-Q1;
    \end{itemize}
    
    \item Breakdown Equ. \ref{equ:attn_op} to show how the matrix multiplication is transformed to $Q \cdot K$.
    \begin{itemize}
        \item \textbf{Where}: Equ. \ref{equ:attn_op}
        \item \textbf{Who}: Reviewer-B-Q4;
    \end{itemize}
    
    \item Clarify why encoder can be pipelined with dense and sparse matrix multiplication.
    \begin{itemize}
        \item \textbf{Where}: Sec. \ref{sec:encoder_and_decoder_engines}
        \item \textbf{Who}: Reviewer-B-Q7;
    \end{itemize}
    
    \item More elaboration for Sec. 5.2.3.
    \begin{itemize}
        \item \textbf{Where}: Sec. \ref{sec:reconfigurability}
        \item \textbf{Who}: Reviewer-B-Q8;
    \end{itemize}
    
    \item More elaboration for Fig. 17 (original manuscript).
    \begin{itemize}
        \item \textbf{Where}: Fig. \ref{fig:ae_levit} and Sec. \ref{sec:alg_exps}
        \item \textbf{Who}: Reviewer-B-Q11;
    \end{itemize}
    
    \item Fix grammar issues.
    \begin{itemize}
        \item \textbf{Where}: Scattered in between Sec. \ref{sec:hardware_motivation}, \ref{sec:micro-arch}, and \ref{sec:exp_setting}
        \item \textbf{Who}: Reviewer-B-Q13;
    \end{itemize}
    
    \item Only show the difference between NLP Transformers and ViTs in the introduction to avoid under-selling the idea.
    \begin{itemize}
        \item \textbf{Where}: Sec. \ref{sec:intro}
        \item \textbf{Who}: Reviewer-C-Q3;
    \end{itemize}
    
    \item Remove the mentioned sentence in Sec. 3.1.
    \begin{itemize}
        \item \textbf{Where}: Sec. \ref{sec:bottlenecks}
        \item \textbf{Who}: Reviewer-C-Q5;
    \end{itemize}
    
    \item Add discussion of extending to NLP Transformer models.
    \begin{itemize}
        \item \textbf{Where}: Sec. \ref{sec:overall_comp}
        \item \textbf{Who}: Reviewer-D-Q1;
    \end{itemize}
    
    \item Add accuracy drop ranges in the abstract.
    \begin{itemize}
        \item \textbf{Where}: Abstract
        \item \textbf{Who}: Reviewer-D-Q6;
    \end{itemize}
    
    \item Revise the description of Alg. \ref{alg:split_and_conquer} to cross reference the line numbers; Similarly, cross reference for Fig. \ref{fig:architecture}.
    \begin{itemize}
        \item \textbf{Where}: Sec. \ref{sec:alg_split_and_conquer} and Sec. \ref{sec:micro-arch}
        \item \textbf{Who}: Reviewer-E-Q2;
    \end{itemize}
    
    \item Show a small example walking through how split and conquer algorithm works.
    \begin{itemize}
        \item \textbf{Where}: Fig. \ref{fig:split_and_conquer}
        \item \textbf{Who}: Reviewer-E-Q6;
    \end{itemize}
\end{itemize}

\end{appendices}
